# Supplementary material for: LINOCS: Lookahead Inference of Networked Operators for Continuous Stability
Source: arXiv:2404.18267 source file (2024-04-28)
Supplement: Supplementary file 1 [file supp_notation_table.tex]

\section{Notation}
\begin{table}[h!]
 \hspace*{-1cm} 
    \caption{List of notations for SiBBLINGS.}
    \begin{tabular}
    {|p{0.2\linewidth}|p{0.7\linewidth}|}     
        \hline        
        \textbf{Symbol} & \textbf{Description} \\
        \hline
        Full lookahead reconstruction & Reconstructing the time-series by iteratively estimating the value in each time point (\(\widehat{\bm{x}}_t\)) using our estimation of the data for the previous time point (\(\widehat{\bm{x}}_{t-1}\)), starting from initial conditions. \\ 
        k-order LINOCS reconstruction  & Reconstructing the time-series by iteratively estimating the value in each time point (\(\widehat{\bm{x}}_t\)) using our estimation of the data for the previous time point (\(\widehat{\bm{x}}_{t-1}\)), starting from $k$ time points to the past ($\bm{x}_{\max{[t-k, 0]}}$). \\
        1-step reconstruction & constructing the time-series by iteratively estimating the value in each time point (\(\widehat{\bm{x}}_t\)) using the \textbf{observed} values at the previous time point (\(\bm{x}_{t-1}\)), \\

        \hline
    \end{tabular}
   
    \label{tab:notations}
\end{table}
